# Supplementary material for: The Influence of Motility on Bacterial Accumulation in a Microporous Channel
Source: arXiv:2009.01605 ancillary file (2020-11-26)
Supplement: Supplementary file 1 [file supplement.pdf]

# Electronic Supplementary Information

Miru Lee*

*Institute for Theoretical Physics, Georg-August-Universität Göttingen, 37073 Göttingen, Germany*

Christoph Lohrmann†

*Institute for Computational Physics, University of Stuttgart,*

*Allmandring 3, 70569 Stuttgart, Germany*

Kai Szuttor

*Institute for Computational Physics, University of Stuttgart,*

*Allmandring 3, 70569 Stuttgart, Germany*

Harold Auradou‡

*Université Paris-Saclay, CNRS, FAST, 91405, Orsay, France*

Christian Holm§

*Institute for Computational Physics, University of Stuttgart,*

*Allmandring 3, 70569 Stuttgart, Germany*

(Dated: November 20, 2020)

* miru.lee@uni-goettingen.de

† clohrmann@icp.uni-stuttgart.de

‡ harold.auradou@universite-paris-saclay.fr

§ holm@icp.uni-stuttgart.de

## I. PARAMETER CHOICE

The parameters for the lattice Boltzmann simulations are:

$$
\begin{aligned}
\text{LB grid spacing:} &\quad \Delta x = 1, \\
\text{LB time step:} &\quad \tau = 1, \\
\text{LB fluid density:} &\quad \rho = 1, \\
\text{LB kinematic viscosity:} &\quad \eta = 0.1, \\
\text{LB bare friction coefficient:} &\quad \xi = 0.25.
\end{aligned}
$$

On top of the LB, the MD simulation is running to compute the swimmers' equations of motions. The effective size of a single bead that occupy the space is realized by the Weeks-Chandler-Andersen (WCA) potential [1]:

$$
\begin{aligned}
\text{MD time step:} &\quad \Delta t = \frac{\tau}{5} = 0.2, \\
\text{Effective diameter of a bead:} &\quad \sigma = \Delta x = 1, \\
\text{WCA potential strength:} &\quad \epsilon = 1, \\
\text{WCA cutoff radius:} &\quad r_0 = 2^{\frac{1}{6}} \Delta x.
\end{aligned}
$$

At a low Reynolds number, the flow velocity scales linearly with the external force density. In the case where the system is $(L, H, W) = (500\,\mu\text{m}, 200\,\mu\text{m}, 20\,\mu\text{m})$ with a periodic boundary condition in the $x$ direction, the average flow speed in the channel $u_{\text{avg}}$ is given by

$$u_{\text{avg}} = 17.7 \times \text{force density}. \tag{1}$$

On the other hand, when the system is constructed as $(L, H, W) = (500\,\mu\text{m}, 500\,\mu\text{m}, 20\,\mu\text{m})$ with a periodic boundary condition in the $x$ and $y$ directions, the average flow speed $u_{\text{avg}}$ scales

$$u_{\text{avg}} = 40.1 \times \text{force density}. \tag{2}$$

As such the swimmer speed is determined by the dipole force strength $f_{\text{dp}}$ with a scaling factor, i.e., the effective friction $\xi_{\text{eff}}$

$$U_{\text{s}} = \xi_{\text{eff}} f_{\text{dp}}, \tag{3}$$

where

$$
\begin{aligned}
U_{\text{s}} &= 6.67 \times 10^{-5} \\
f_{\text{dp}} &= 7.52 \times 10^{-5} \\
\xi_{\text{eff}} &= 0.89.
\end{aligned} \tag{4}
$$

The dimensionless parameters above can be related to those of the experiment done by Miño et al. by specifying conversion factors for the length $C_s$, time $C_t$, and mass $C_m$.

Starting with the length conversion factor, we match the radius of the obstacle:

$$\text{Radius:} \quad R = 32\sigma = 80\,\mu\text{m},$$

which yield us the length conversion factor:

$$C_x = 2.5\,\mu\text{m}.$$

The mass conversion factor can be found by matching the LB fluid density with the density of water:

$$10^{-15}\,\text{kg}/\mu\text{m}^3 = 1C_\rho = 1\frac{C_m}{C_x^3}$$
$$\rightarrow C_m = 1.56\times 10^{-14}\,\text{kg}.$$

The last conversion factor, the time, can be found by comparing the time scales of the simulation and the experiment. We relate the swimmer's swimming velocity. *E.coli* bacteria swim at around $24\,\mu\text{m/s}$. In our simulations, our swimmers swim at $U_\text{S} = 6.67\times 10^{-5}\frac{C_m}{C_\tau}$, thus the time conversion factor is

$$24\,\mu\text{m/s} = 6.67\times 10^{-5}\frac{C_m}{C_\tau}$$
$$\rightarrow C_\tau = 6.94\times 10^{-6}\,\text{s}.$$

Note that this time conversion factor is 10 times larger than the value that one would have obtained via the viscosity of water. This is because we scale up the velocities of the experiment by a factor of 10. It is possible as long as the system is at sufficiently low Reynolds numbers (Re). Our simulation and the experiment show $\text{Re} \sim 10^{-2}$ and $\sim 10^{-3}$, respectively.

These three conversion factors uniquely map any number that carry a dimensionality in our simulation to its physical counterpart.

## II. VIDEOS

We include three videos to supplement our arguments. These videos show three different running durations $T_\text{r} \in \{0.3, 3.7, 21\}$, whose filenames are `S1_Trun_0_3.mp4`, `S2_Trun_3_7.mp4`, and `S3_Trun_21.mp4`, respectively. The other parameters are kept the same.

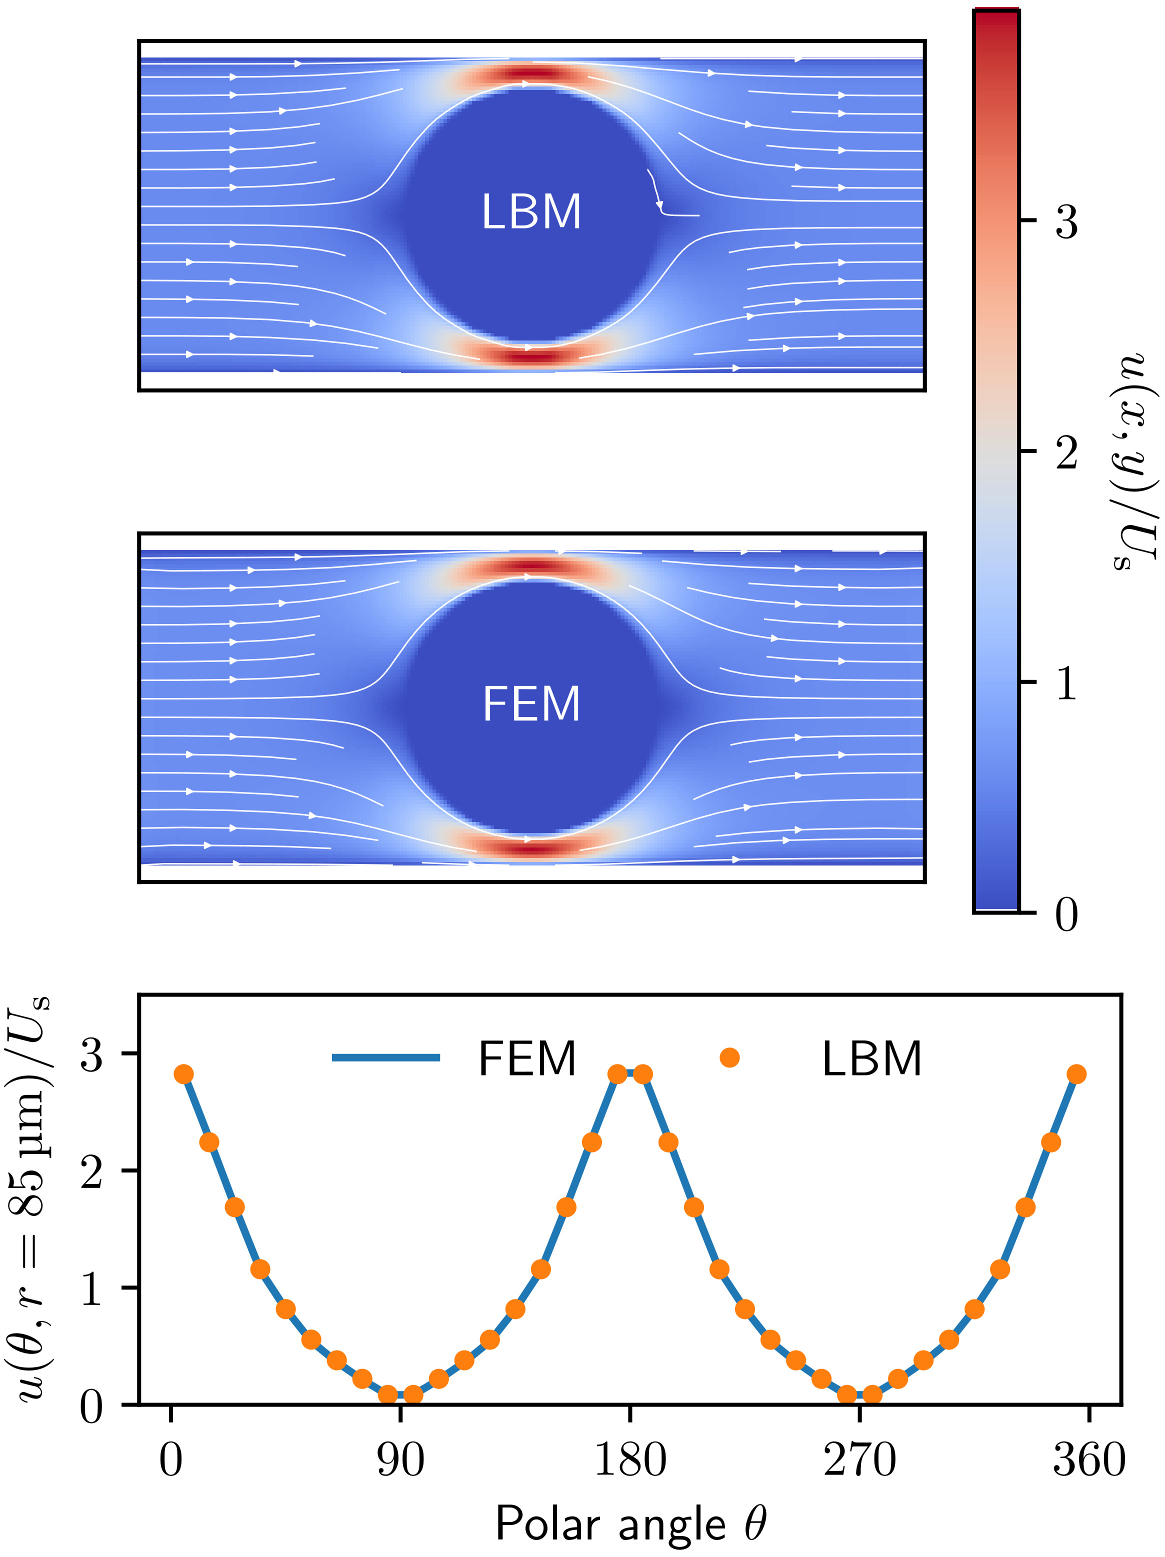


FIG. 1. A flow field comparison between a Lattice-Boltzmann Method (LBM) simulation and Finite Element Method (FEM) simulation. The upper plot shows the flow fields projected to the $xy$ plane from both simulations. The lower plot qualitatively compares the flow strength around the obstacle as a function of the polar angle $\theta$.

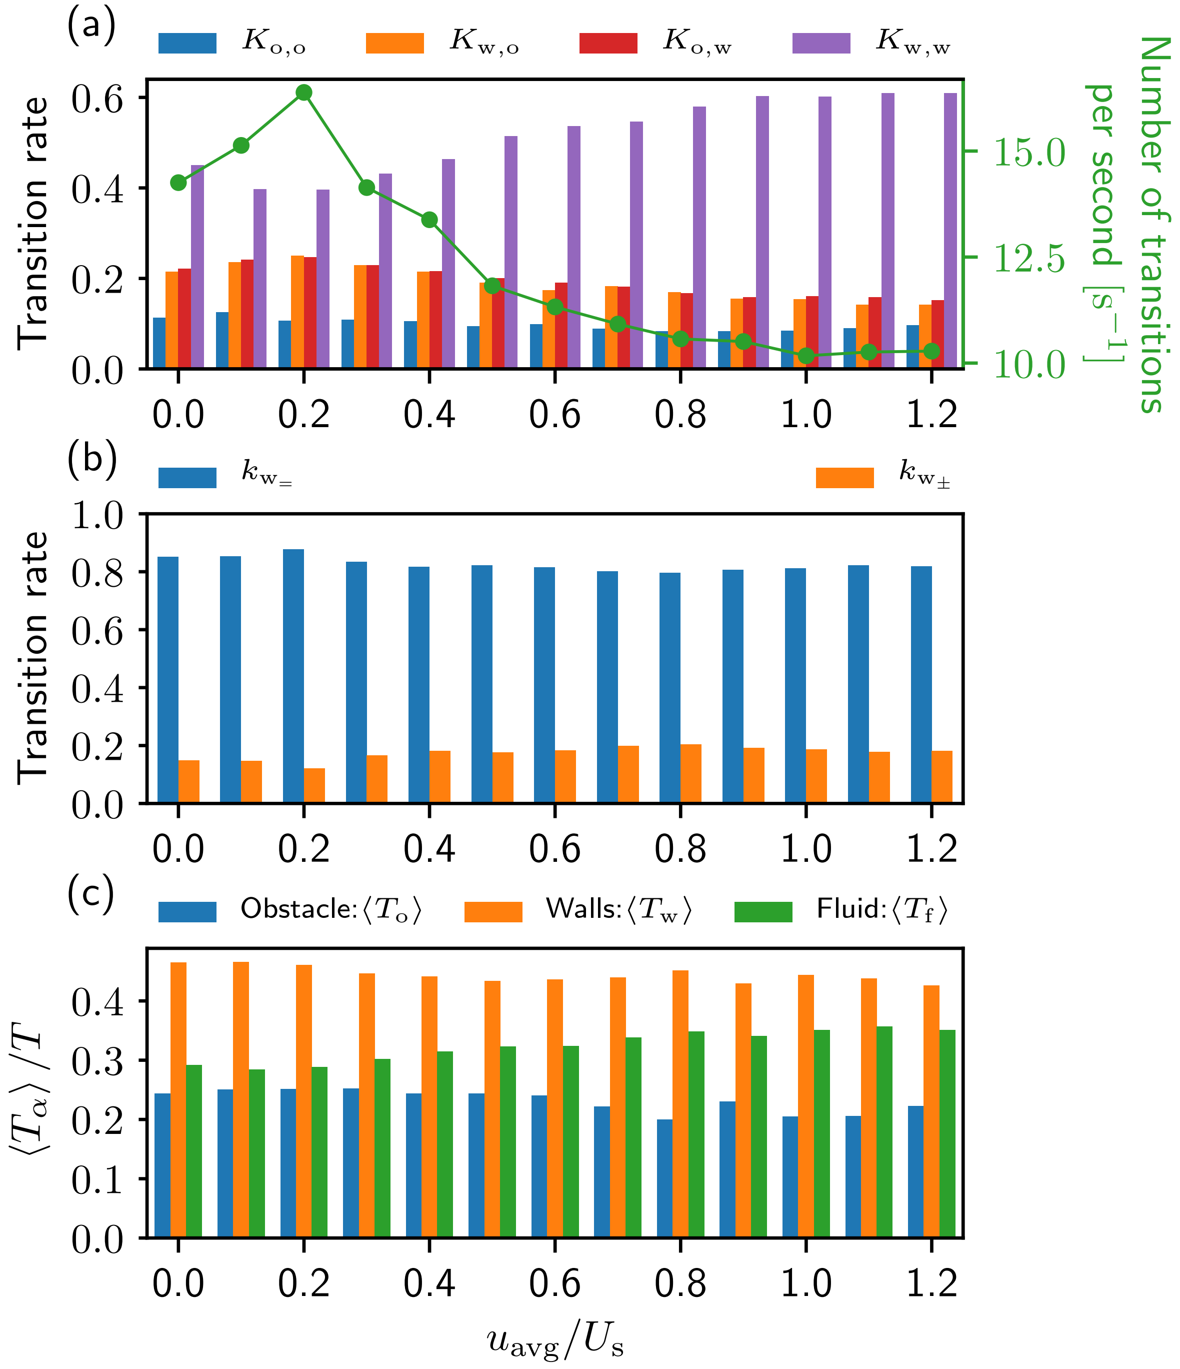


FIG. 2. (a): $K_{i,j}$ refers to a transition rate from $i$ to $j$ with $i, j \in$ {o,w}. "o" and "w" denote the obstacle and the wall, respectively. The green curve represents the total number of the transitions per second. (b): dissecting $K_{w,w}$ into two parts; the trivial transition between the same wall $k_{w_=}$ and the migration between the upper and lower walls $k_{w_\pm}$. (c): it shows the average time spent on/in $\alpha$, $\langle T_\alpha \rangle$, with $\alpha \in$ {o,w,f} indicating the obstacle, the walls, and the fluid. $T$ is the total measurement time. All the data are plotted as a function of the external flow strength.

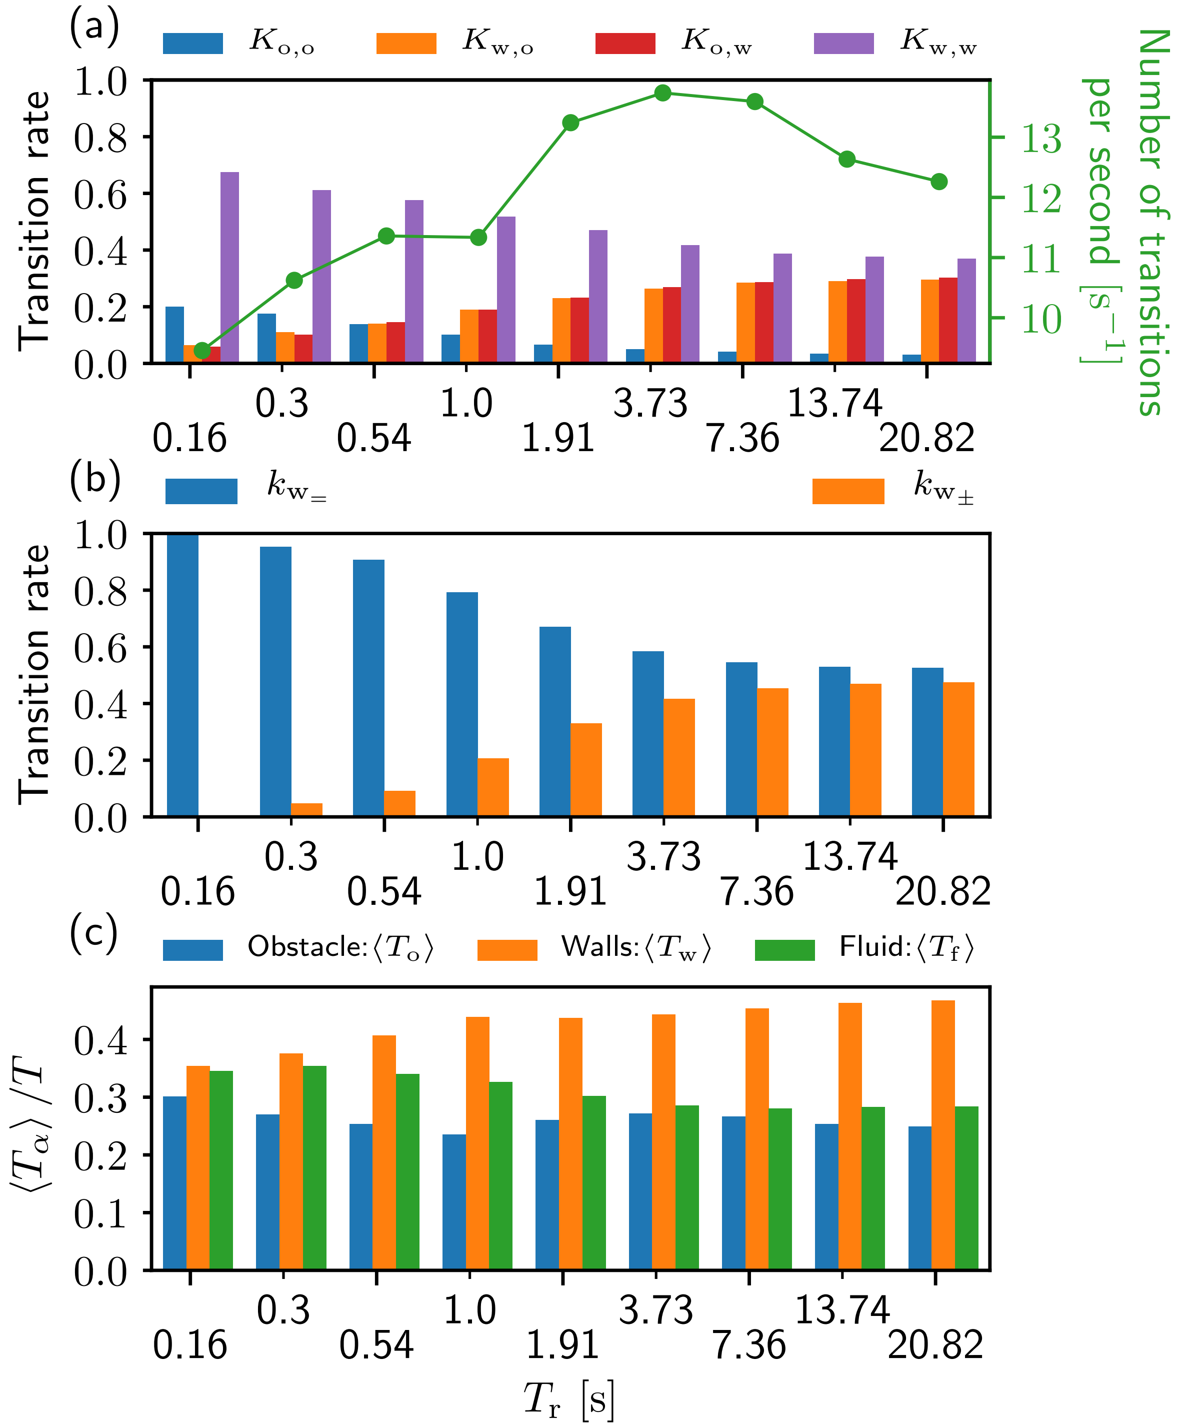


FIG. 3. (a): $K_{i,j}$ refers to a transition rate from $i$ to $j$ with $i, j \in$ {o,w}. "o" and "w" denote the obstacle and the wall, respectively. The green curve represents the total number of the transitions per second. (b): dissecting $K_{w,w}$ into two parts; the trivial transition between the same wall $k_{w_=}$ and the migration between the upper and lower walls $k_{w_\pm}$. (c): it shows the average time spent on/in $\alpha$, $\langle T_\alpha \rangle$, with $\alpha \in$ {o,w,f} indicating the obstacle, the walls, and the fluid. $T$ is the total measurement time. All the data are plotted as a function of the (average) running duration $T_{\mathrm{r}}$.

[1] J. D. Weeks, D. Chandler, and H. C. Andersen. Role of repulsive forces in determining the equilibrium structure of simple liquids. *The Journal of Chemical Physics*, 54:5237, 1971.

[2] Gastón L. Miño, Magali Baabour, Ricardo Chertcoff, Gabriel Gutkind, Eric Clément, Harold Auradou, and Irene Ippolito. E coli accumulation behind an obstacle. *Advances in Microbiology*, 8:451–464, 2018. doi:10.4236/aim.2018.86030.
